# Supplementary material for: Contrastive Object Detection Using Knowledge Graph Embeddings
Source: arXiv:2112.11366 source file (2021-12-21)
Supplement: Supplementary file 1 [file supplementary.tex]

%%%%%%%%% TITLE
\title{Contrastive Object Detection Using Knowledge Graph Embeddings \\ \textit{Supplementary Material}}
%https://openaccess.thecvf.com/content_CVPR_2020/supplemental/Roth_PADS_Policy-Adapted_Sampling_CVPR_2020_supplemental.pdf

\author{Christopher Lang$^{1,2}$, Alexander Braun$^{1}$, and Abhinav Valada$^{2}$% <-this % stops a space
\thanks{$^{1}$Robert Bosch GmbH, Germany}%
\thanks{$^{2}$Department of Computer Science, University of Freiburg, Germany}%
\tt\small\{riverav, hurtadoj, valada\}@cs.uni-freiburg.de}

\maketitle
In this supplementary material, we provide additional experimental results that support the novelty of the contributions made and evaluate our architectural design choices. Particularly, we first provide further details regarding the data collection methodology of our Multimodal Audio-Visual Detection (MAVD) dataset in \secref{sec:SM_sensor}. We then compare the performance of different EfficientDet variants in our proposed MM-DistillNet framework in \secref{sec:SM_EfficientDet}. In \secref{sec:SM_microphones}, we evaluate the performance of our framework with sound from a varying number of microphones as input. Subsequently, we demonstrate the capabilities of our multi-teacher single-student framework to distill knowledge from RGB images into other modalities that are complementary to sound in \secref{sec:SM_modalities}. We then present ablation studies on the influence of various hyperparameters in our proposed MTA loss function in \secref{sec:SM_hyperP} and we compare the performance of our MTA loss with other widely employed knowledge distillation losses in \secref{sec:SM_loses}. Subsequently,  we present additional results on our proposed self-supervised pretext task for the audio student in \secref{sec:SM_pretext}. Then, we present results of our framework in low illumination conditions such as nighttime and dusk in \secref{sec:SM_scenarios}. Finally, we extend our qualitative results with numerous examples in \secref{sec:qualitativeS}. We made the code and models of our approach publicly available at \url{http://rl.uni-freiburg.de/research/multimodal-distill}.\blfootnote{*Equal contribution}\blfootnote{The authors would like to thank Johan Vertens for assistance in the data collection.}
%%%%%%%%% BODY TEXT

\section{Extended Ablation Study}

\subsection{EfficientDet Compound Coefficient Selection}
\label{sec:SM_EfficientDet}

EfficientDet is a family of object detection models proposed by 
Tan~\textit{et~al.}~\cite{tan2020efficientdet} which contains eight different architectural configurations that trade-off performance and runtime. We evaluated the performance of the variants to identify their suitability for our framework. To this end, we created a large dataset by combining Microsoft~COCO~\cite{lin2014microsoft}, PASCAL~VOC~\cite{everingham2010pascal}, and ImageNet~\cite{deng2009imagenet}. Subsequently, we removed all the scenes that do not contain at least one vehicle and retained the bounding boxes of those that contain cars or moving vehicles. We then trained EfficientDet~D0-D7 to detect the objects in this combined dataset. In \tabref{table:efficientdetruntimes}, we present the performance in terms of the Average Precision (AP) at $IoU=0.5$, as well as the inference time and the Floating Point Operations Per Second (FLOPS). We chose EfficientDet~D2 as the backbone of our framework, given that it presents a higher improvement in the average performance with a lesser increase in the inference time. Nevertheless, our framework provides the flexibility to adopt any of the other variants as a direct drop in replacement.

\begin{table}
\begin{center}
\footnotesize
\begin{tabular}{p{1.8cm}|p{1cm}p{1cm}p{1.2cm}}
\toprule
EfficientDet Variant & AP@ 0.5 & FLOPS & Inference Time (\si{\milli\second}) \\
\noalign{\smallskip}\hline\hline\noalign{\smallskip}
D0 & 0.5165 & 2.5B & 30.04 \\
D1 & 0.6870 & 6.1B& 34.76 \\
\textbf{D2} & \textbf{0.7974} & \textbf{11B} & \textbf{39.99} \\
D3 & 0.8134 & 25B& 59.45 \\
D4 & 0.8680 & 55B& 89.93 \\
D7 & 0.9200 & 325B& 388.90\\
\bottomrule
\end{tabular}
\end{center}
\caption{Performance comparison of different EfficientDet variants for predicting bounding boxes of vehicles in Microsoft COCO~\cite{lin2014microsoft}, PASCAL~VOC~\cite{everingham2010pascal}, and ImageNet~\cite{deng2009imagenet}, with the associated AP at 0.5 IoU.}
\label{table:efficientdetruntimes}
\end{table}

\subsection{Influence of Number of Microphones}
\label{sec:SM_microphones}

\pgfplotsset{width=7cm,compat=1.3}
\begin{figure}
    \footnotesize
    \centering
    \begin{tikzpicture}
    \pgfplotsset{
        xmin=2, xmax=8,
    }

    \begin{axis}[
        axis y line*=left,
        ymin=0, ymax=40,
        xlabel = Number of Microphones,
        ylabel = mAP@Avg,
        grid=both,
        height = 5.5cm,
        width =\linewidth,
        every axis plot/.append style={very thick}
    ]
        \addplot[red]
        coordinates {
          (2,  23.1255)
          (4,  23.47)
          (6,  26.0511)
          (8, 26.487)
        };\label{microphoneAP}
    \end{axis}
    
    \begin{axis}[
        axis y line*=right,
        axis x line=none,
        ymin=0, ymax=0.50,
        ylabel=GFLOPS,
        height = 5.5cm,
        width =\linewidth,
        every axis plot/.append style={very thick}
    ]
    \addlegendimage{/pgfplots/refstyle=microphoneAP}\addlegendentry{Microphone mAP}
        \addplot[blue]
        coordinates {
          (2,  0.00)
          (4,  0.13)
          (6,  0.17)
          (8, 0.21)
        };\addlegendentry{Increase in FLOPS}
    \end{axis}
    
    \end{tikzpicture} 
    \caption{The left axis (blue line) shows the performance of the network vs the number of microphones. The right axis (red) shows the GLOPS increase caused by using N microphones. It can be seen, that more channels improve the performance in the given task with negligible impact in FLOPS.}
    \label{fig:mics}
\end{figure}

Our proposed MM-DistillNet framework exploits complementary cues from different modalities such as RGB, depth, and thermal images during training to incorporate multimodal information into a single audio network. The input to the audio network is from a microphone array that captures ambient sounds. We employ multiple monophonic microphones due to the promising results that it has demonstrated for sound source localization~\cite{ma2019phased}. \figref{fig:sensors} shows the microphone array that we employ mounted on our data collection vehicle. In order to estimate the number of microphones that are essential to reliably localize objects, we analyze the performance of our MM-DistillNet for varying number of microphones in a balanced subset of the dataset.

Namely, we hypothesize that there is a relationship between the number of microphones and the complexity of the scene, as measured by the number of vehicles in the environment. Our MAVD dataset contains varying number of vehicles in each scene, with a maximum of 13 vehicles in a single scene. We performed experiments to analyze the improvement that we can achieve by using more number of microphones in the array. To do so, we need to have balanced number of vehicles in the dataset. Therefore, we apply an under-sampling approach to ensure that the number of examples with varying number of vehicles are balanced. We compute the performance of the audio student using multiples of two number of microphones, in order to always consider the microphones that are further away from each other in the hexagonal array.

\figref{fig:mics} shows that increasing the number of microphones consistently improves the performance of the model. Therefore, we utilize sound from all the eight monophonic microphones that are available in our octagonal setup for our experiments. Nevertheless, given that each microphone adds an additional $768\times768\times1$ input to the network, we computed the additional overhead in terms of the increase in number FLOPS in the network. \figref{fig:mics} shows that the increase in FLOPS in the network due to the addition of a microphone is negligible compared to the overall FLOPS of EfficientDet as shown in \tabref{table:efficientdetruntimes}.
    
\subsection{Distillation to Different Student Modalities}
\label{sec:SM_modalities}

\begin{table}
\begin{center}
\footnotesize
\begin{tabular}{p{2.5cm}p{1.2cm}|p{1.35cm}}
\toprule
Teachers & Student & mAP@ Avg  \\
\noalign{\smallskip}\hline\hline\noalign{\smallskip}
%RGB & Sound & $44.57$ \\
RGB & Sound & $57.25$ \\
RGB & Thermal & $56.70$ \\
\midrule
RGB, Depth, Thermal & Sound & $61.62$ \\
RGB, Depth, Thermal & RGB & $81.12$ \\
RGB, Depth, Thermal & Thermal & $\mathbf{81.98}$ \\
\bottomrule
\end{tabular}
\end{center}
\caption{Our framework distills the knowledge from multimodal teachers trained on dataset where supervision is available, to improve the learning of a single student network. Thermal and RGB modalities show significant improvement over their single teacher counterparts.}
\label{table:nonaudio}
\end{table}

By taking advantage of the co-ocurrence of all the modalities present in our dataset (audio, RGB, thermal and depth), it is straightforward to interchange the input modality of the student network from audio to any of the other modalities as described in Sec.~3 of the main paper. By doing so, we can exemplify not only how our method is modality independent, but also how it can further improve the performance of existing object detection frameworks.

In the other experiments, we selected RGB, depth, and thermal images as the teacher modalities and sound as the student modality for our framework. This enables us to tackle limitations of visual modalities such as occlusions and sensor sensitivity (poor performance of RGB cameras during nighttime as well as the limited sensitivity of thermal cameras during the day). Nevertheless, our approach to transfer the knowledge from multiple pre-trained modality-specific networks to a student network, is input agnostic. Under this perspective, instead of employing sound as input to the student network, we can also use conventional RGB, depth, or thermal modalities as input to our framework. \tabref{table:nonaudio} presents results with different modalities as input to the student network. It can be seen that the performance against the single teacher is substantially improved. Particularly, using the thermal modality as input to the student network provides the best performance, as it provides substantial cues for vehicle detection in both day as well as night recordings. Whereas, using RGB as input to the student during night suffers due to low illumination conditions. Nevertheless, using a thermal modality requires expensive hardware and is subject to visual limitations like occlusion. For this reason, we employ audio in our MM-DistillNet as an alternative to the traditional visual inputs used in autonomous driving.

\subsection{Influence of Hyperparameters in MTA Loss}
\label{sec:SM_hyperP}

We define our proposed Multi-Teacher Alignment (MTA) loss function as
\begin{equation}
\label{eq:MTAloss}
L_{MTA} = \beta * \sum_{j} KL_{div}\left(\frac{Q_{s}^j}{\left \|  {Q_{s}^j}\right \|_{2}}, \frac{Q_{t}^j}{\left \| {Q_{t}^j}\right \|_{2}}\right),
\end{equation}
where $Q_{s}^j = F_{avg}^{r}(A_{s})$ and $Q_{t}^j = \prod_{i}^{N} F_{avg}^{r}(A_{t_{i}})$ are the student and multi-teacher attention maps respectively. Additionally, while computing the $KL_{div}$ as a measure of the difference between probability distributions between the teachers and the student, we can apply a temperature $t$ to the softmax as proposed by Hinton~\textit{et~al.}~\cite{hinton2015}. This temperature in the softmax computation is added to adapt the confidence on each individual probability distribution. To this end, we can expand the above notation using the student normalized activation $S_{x}=\frac{Q_{s}^j}{\left \|  {Q_{s}^j}\right \|_{2}}$ and the integrated normalized teacher attention $T_{x}=\frac{Q_{t}^j}{\left \| {Q_{t}^j}\right \|_{2}}$ as
\begin{equation}
\label{eq:klexpanded}
KL_{div}\left(S_{x}||T_{x}\right)= \sum_{x \in \mathcal{X}}\frac{e^{\frac{S_{x, i}}{t}}}{\sum_{k=1}^{n} e^{\frac{S_{x,k}}{t}}} \log \left(\frac{\frac{e^{\frac{S_{x, i}}{t}}}{\sum_{k=1}^{n} e^{\frac{S_{x,k}}{t}}}}{\frac{e^{\frac{T_{x, i}}{t}}}{\sum_{k=1}^{n} e^{\frac{T_{x,k}}{t}}}}\right)
\end{equation}

We employ this loss in addition to the focal loss $L_{focal}$ to optimize our MM-DistillNet framework as
\begin{equation}
\label{eq:totallossS}
L_{total} = \delta * L_{focal} + \omega * L_{MTA}.
\end{equation}

With this formulation, we have two hyperparameters in the MTA loss function that can be selected according to the specific task: the exponential value $r$, which controls the relevance of small valued activations in contrast to large valued activations, and the softmax temperature $t$. We performed experiments to study the influence of these two hyperparameters on the performance of the audio student network. Results from this experiment is shown in \tabref{table:losshyper}. We present the mean average precision of our best recipe using a single RGB teacher and the audio student network. 

\begin{table}
\begin{center}
\footnotesize
\begin{tabular}{p{1.5cm}p{1.5cm}|p{1.4cm}}
\toprule
r & t & mAP@ Avg \\
\noalign{\smallskip}\hline\hline\noalign{\smallskip}
4          & 9          & 60.13       \\
4          & 6          & 61.40       \\
3          & 4          & 64.08       \\
3          & 2          & 64.30       \\
2          & 6          & 64.30       \\
2          & 4          & 66.05       \\
2          & 7          & 66.43       \\
1          & 3          & 67.68       \\
1          & 4          & 67.74       \\
1          & 9          & 69.67       \\
2          & 9          & $\mathbf{69.72}$ \\
\bottomrule
\end{tabular}
\end{center}
\caption{Ablation study of hyperparameters $r$ and temperature $t$ in the proposed MTA loss function. The object detection performance is shown for an audio student with knowledge distilled from a RGB teacher network.}
\label{table:losshyper}
\end{table}

We observe that in this setting, a value of $r=4$ and $t=9$ provides the best result. This suggests that putting more importance to higher valued activations rather than low-valued activations improves the overall performance of the network. 

\subsection{Ranking Loss vs. MTA Loss}
\label{sec:SM_loses}

\begin{table}
\begin{center}
\footnotesize
\begin{tabular}{p{1.2cm}|p{2cm}|p{2cm}}
\toprule
Input & \multicolumn{2}{c}{mAP@ Avg} \\
\cmidrule{2-3}
 & Ranking Loss~\cite{gan2019self} & MTA Loss (Ours) \\
\noalign{\smallskip}\hline\hline\noalign{\smallskip}
RGB & 56.37 & $\mathbf{57.25}$ \\
Thermal & 55.82 & $\mathbf{56.70}$ \\
Depth & 45.85 & $\mathbf{55.41}$ \\
\bottomrule
\end{tabular}
\end{center}
\label{table:singleteacherourloss}
\caption{Our MTA loss function was formulated to distill knowledge from multiple teachers to a single student. Nevertheless, it yields superior performance than Ranking loss employed by Gan~\textit{et~al.}~\cite{gan2019self} for knowledge distillation in a single teacher-student scenario.}
\end{table}

The proposed MM-DistillNet framework exploits the co-occurrence of different modalities representing a scene. Our MTA loss facilitates this process by aligning the intermediate representations of multiple teachers to that of a single student. The previous state-of-the-art~\cite{gan2019self} method employs the Ranking loss to distill knowledge from a single teacher to a single student network. To further demonstrate the capabilities of our proposed MTA loss, we compare its performance with Ranking loss for distillation of knowledge from a single modality-specific teacher to an audio student network. We performed this experiment for all the teacher modalities considered in this work. Although our loss function is designed to align different intermediate representations of modality-specific networks, we observe that it outperforms the Ranking loss formulation even in the single teacher setting.\looseness=-1

\section{Evaluation of Audio Student Pretext Task}
\label{sec:SM_pretext}

\begin{figure}
    \footnotesize
    \centering
\begin{tikzpicture}
    \pgfplotsset{
        xmin=0, xmax=27,
    }
    \begin{axis}[
        axis lines = left,
        xlabel = Epochs,
        ylabel = $L_{total}$,
        grid=both,
        height = 5.5cm,
        width =\linewidth,
        every axis plot/.append style={very thick}
    ]
        \addplot coordinates {
          (1,  0.8637468)
          (6,  0.5210465)
          (11,  0.138963)
          (16, 0.04530995)
          (21, 0.008364)
          (26, 0.004460582)
        };
        \addlegendentry{No Pretext Task}
        \addplot coordinates {
          (1,  0.49357)
          (6,  0.105744)
          (11,  0.027559)
          (16, 0.016903)
          (21, 0.005821)
          (26, 0.003497)
        };
        \addlegendentry{With Pretext Task}
    \end{axis}
    \end{tikzpicture} 
    \caption{Comparison of training convergence of our MM-DistillNet, with and without the initialization of the student network with weights of the model trained on our proposed self-supervised pretext task.}
    \label{fig:pretext}
\end{figure}

Our MM-DistillNet contains multiple modality-specific teachers and a single student network. Each of the networks are composed of the EfficientNet backbone which has to be initialized with pre-trained weights from large datasets to ease the optimization and achieve better convergence. Since all existing pre-trained models of EfficientNet primarily employ 3-channel RGB images as input, they cannot be used for initializing the audio student network which takes 8-channel spectrograms as input (1-channel spectrogram from each of the 8 microphones in the array). To address this problem, we propose a self-supervised pretext task that provides the audio student network with semantically rich information about the relationship between the audio and visual modalities. The goal of the pretext task is to estimate the number of vehicles present in the RGB image only using sound as input to the network. In the ablation study presented in the main paper, we show that our proposed pretext task improves the performance in terms of detection metrics. In \figref{fig:pretext} of this supplementary material, we present comparisons of the training curves for the MM-DistillNet framework, with and without the initialization of the audio student network with weights of the model trained on the proposed pretext task. We can see that the model with weighted initialized from the pretext task consistently yields a lower loss since the early stages. Moreover, the final loss is $27.55\%$ lower than the model trained from scratch. These results demonstrate that the pretext task not only improves the performance in terms of the metrics, it also accelerates training and leads to faster convergence.

\section{Evaluation in Low Illumination Conditions}
\label{sec:SM_scenarios}

\begin{table*}
\begin{center}
\footnotesize
\begin{tabular}{p{1.2cm}|p{1.5cm}|p{2.5cm}|p{1cm}p{1cm}p{1cm}p{0.8cm}p{0.5cm}}
\toprule
Condition & Vehicle State & Network & mAP@ Avg & mAP@ 0.5 & mAP@ 0.75 & CDx & CDx \\
\noalign{\smallskip}\hline\hline\noalign{\smallskip}
Day & Static & StereoSoundNet~\cite{gan2019self} & $53.48$ & $69.10$ & $52.50$ & $2.77$ & $1.51$ \\
Night & Static & StereoSoundNet~\cite{gan2019self} & $38.13$ & $49.26$ & $34.67$ & $4.34$ & $3.95$ \\
Day & Driving & StereoSoundNet~\cite{gan2019self} & $45.59$ & $69.20$ & $42.84$ & $2.50$ & $1.60$ \\
Night & Driving & StereoSoundNet~\cite{gan2019self} & $28.56$ & $45.18$ & $24.43$ & $3.86$ & $2.77$ \\
\midrule
Day & Static & MM-DistillNet & $63.80$ & $83.90$ & $63.63$ & $1.59$ & $0.78$ \\
Night & Static & MM-DistillNet & $75.10$ & $89.63$ & $73.23$ & $1.43$ & $0.70$ \\
Day & Driving & MM-DistillNet & $55.73$ & $81.51$ & $52.75$ & $1.24$ & $0.76$ \\
Night & Driving & MM-DistillNet & $48.13$ & $67.16$ & $46.07$ & $1.93$ & $1.50$ \\
\bottomrule
\end{tabular}
\end{center}
\vspace{-0.2cm}
\caption{Performance comparison of MM-DistillNet in different illumination conditions as well as driving and static (data collection vehicle) states. Our framework outperform the previous state-of-the-art even in static-day conditions, where the RGB teacher performs the best.}
\label{table:resultsdiffconditions}
\end{table*}

In this section, we compare the performance our proposed MM-DistillNet and the previous state-of-the-art StereoSoundNet~\cite{gan2019self} in different illumination and driving conditions. StereoSoundNet is trained under the supervision of the RGB teacher, whereas our MM-DistillNet uses the RGB, depth, and thermal teachers. \tabref{table:resultsdiffconditions} presents results in terms of the average precision metric for each of these conditions. We can see that in every scenario our proposed MM-DistillNet substantially outperforms StereoSoundNet, thereby achieving state-of-the-art performance. We observe the largest improvement during night time conditions where StereoSoundNet significantly falls behind. It can also be observed that even during the day when the data collection vehicle is not in motion, our MM-DistillNet achieves over $10\%$ improvement in the mAP @ Average. We observe a performance drop in both the methods from static to driving conditions, which can be attributed to the distortion of sound due to the moving data collection vehicle, wind on the microphone (note that the microphones in the array were not equipped with a wind muff) and high ambient noise conditions. We believe that high fidelity microphones and hard negative mining will help overcome this problem. This experiment demonstrates that incorporating knowledge from multiple modality-specific teachers improves the performance of the audio student, especially while the data collection vehicle is in motion and in low illumination conditions. 

\section{Extended Qualitative Results}
\label{sec:qualitativeS}

In this section, we extend the qualitative evaluations of our proposed MM-DistillNet. We provide further results that demonstrate that our MM-DistillNet effectively employs the knowledge of diverse multimodal pre-trained teachers to improve the performance of vehicle detection. We first highlight how the audio modality is able to overcome the visual limitation by detecting occluded cars in \figref{fig:SM_qualitativeoccluded} where the white car at time $t$ is occluded by the vehicle that appears on the left at $t+1$. However, StereoSoundNet fails to detect the foreground car, while our MM-DistillNet precisely detects both the vehicles in the scene, despite the background car not being visible.

In \figref{fig:SM_qualitativenight}, we present comparison of both methods during nighttime where poor light conditions can be observed. Our MM-DistillNet simultaneously detects multiple cars, even the distant ones, while StereoSoundNet often fails to detect beyond one vehicle. These results demonstrate the novelty of distilling multimodal knowledge in our MM-DistillNet as it shows substantial robustness in poor light conditions, thereby successfully overcoming the limitations of distilling knowledge only from RGB images. Additionally, we qualitatively evaluate the performance of detecting multiple vehicles simultaneously in \figref{fig:SM_qualitativegoodmultiplecars}. Simultaneously detecting multiple vehicles with only sound is an extremely challenging task due to its low spatial resolution. By distilling knowledge from multiple modality-specific teachers, we show that it is not only feasible to detect vehicles simultaneously without relying on the arduous data labeling process, the performance of the detections also substantially improves. Further enhancing this ability will enable a broad spectrum of applications of these audio approaches in real world scenarios. Even though our MM-DistillNet is able to provide very promising results for object detection and tracking, the audio modality suffers from limitations of its own that are highlighted in examples shown in \figref{fig:SM_qualitativefailure}. We observe that occasionally, distant objects are not detected and multiple distant objects are detected as a single object. We believe that a microphone with better sensitivity as well as more examples of this phenomena in the training set will enable our approach to improve the performance in these conditions. Finally, we compare the performance of our MM-DistillNet and the modality-specific RGB, depth, and thermal teachers in \figref{fig:SM_qualitative}. The results show the weaknesses and strengths of each of the selected modalities. Especially in night scenarios, we can observe how the thermal teacher contributes to the distillation of knowledge to the audio student as it reliably detects cars that are not visible in the RGB images, due to low illumination conditions.

% Secuence:
% Detects car before appearing in the visual frame:
% drive_day_2020_05_29_17_43_47_1590767345_965002320_0_image_Prediction_Resized.jpg
%     \includegraphics[width=\linewidth]{images/qualitative_sm/drive_day_2020_05_29_%17_43_47_1590767345_965002320_0_image_Prediction_Resized.baseline.pdf} &  %\includegraphics[width=\linewidth]{images/qualitative_sm/drive_day_2020_05_29_17_43%_47_1590767345_965002320_0_image_Prediction_Resized.ours.pdf} \\
%% drive_day_2020_05_29_17_43_47_1590767350_515357136_0_image_Prediction_Resized.jpg
%     \includegraphics[width=\linewidth]{images/qualitative_sm/drive_day_2020_05_29_%17_43_47_1590767350_515357136_0_image_Prediction_Resized.baseline.pdf} &  %\includegraphics[width=\linewidth]{images/qualitative_sm/drive_day_2020_05_29_17_43%_47_1590767350_515357136_0_image_Prediction_Resized.ours.pdf} \\
%% drive_day_2020_05_29_17_43_47_1590767352_722203864_0_image_Prediction_Resized.jpg
%     \includegraphics[width=\linewidth]{images/qualitative_sm/drive_day_2020_05_29_%17_43_47_1590767350_515357136_0_image_Prediction_Resized.baseline.pdf} &  %\includegraphics[width=\linewidth]{images/qualitative_sm/drive_day_2020_05_29_17_43%_47_1590767350_515357136_0_image_Prediction_Resized.ours.pdf} \\
%\FloatBarrier
